# Supplementary material for: LUT-NN: Empower Efficient Neural Network Inference with Centroid Learning and Table Lookup
Source: arXiv:2302.03213 source file (2023-09-06)
Supplement: Supplementary file 1 [file appendix.ae.tex]

\appendix
\section{Artifact Appendix}

\subsection{Abstract}

In this artifact evaluation appendix, we provide the environmental settings for LUT-NN. We also provide detailed instructions to reproduce the experiment results of LUT-NN.

\subsection{Artifact check-list (meta-information)}

{\small
\begin{itemize}
  \item {\bf Algorithm:} LUT-NN
  \item {\bf Compilation:} Android NDK 21.4.7075529
  \item {\bf Model:} ResNet18, SENet18 and VGG11
  \item {\bf Data set:} CIFAR10, GTSRB, Speech Commands, SVHN, ImageNet and GLUE
  \item {\bf Run-time environment:} Python 3.10
  \item {\bf Hardware:} GPUs for training LUT-NN. x86 CPUs and ARM CPUs for performance evaluation.
  \item {\bf Metrics:} Accuracy, latency (Milliseconds), power (Watt), and memory (Bytes)
  \item {\bf Output:} Output to file
  \item {\bf Experiments:} To train LUT-NN, please follow the training recipes described in the paper.
  To evaluate LUT-NN on accuracy, latency, power and memory, please refer to the experiment workflow section.
  \item {\bf How much disk space required (approximately)?:} 200 GB (Including datasets such as ImageNet)
  \item {\bf How much time is needed to complete experiments (approximately)?: } The performance evaluation takes around 3 hours. To check the number of training hours of LUT-NN, please refer to the table in the \href{https://github.com/lutnn/blink-mm/blob/main/blink_mm/ae/training_recipes.md}{LUT-NN training recipes}.
  \item {\bf Publicly available?:} Yes
  \item {\bf Code licenses (if publicly available)?: } MIT license
  \item {\bf Archived (provide DOI)?:} Not archived temporarily
\end{itemize}
}

\subsection{Description}

\subsubsection{How to access}

We have prepared an artifact evaluation server for reviewers to log in and then evaluate LUT-NN artifacts.
We also make our code repositories public at https://github.com/lutnn.

\paragraph{The AE Server}
The server connects to one Pixel4 phone and another Pixel6 phone through Android Debug Bridge (ADB).
To connect to the evaluation server,
please use SSH.
Firstly, paste the following configuration to .ssh/config:

\begin{lstlisting}
Host jump
    HostName 20.222.121.63
    User ubuntu
    ForwardAgent yes

Host AE-2
    HostName 127.0.0.1
    Port 10002
    User ubuntu
    ProxyJump jump
    ForwardAgent yes
\end{lstlisting}

Secondly, you can connect to the AE-2 server through ``ssh AE-2''.
The password for 20.222.121.63 is ``We're\#1We're\#1'' and the password for 192.168.1.2 is ``We're\#1''.

\subsubsection{Hardware dependencies}

The evaluation of LUT-NN depends on three pieces of hardware: one x86 CPU and two different ARM CPUs.
The AE server satisfies the aforementioned dependency.
The AE server itself is equipped with one Intel x86 CPU (Intel(R) Core(TM) i7-8665U CPU @ 1.90GHz).
It also connects to one Pixel4 phone and one Pixel6 phone through ADB.

\subsubsection{Software dependencies}

\paragraph{Operating Systems}
The AE server has Ubuntu 22.04 installed.
The Pixel4 and Pixel6 have Android 10 and Android 12 installed respectively. 

\subsubsection{Datasets}

This paper uses several datasets to evaluate the performance of LUT-NN.
The datasets are CIFAR10, GTSRB, Speech Commands, SVHN, ImageNet, and GLUE.

\subsubsection{Models}

The models to evaluate are ResNet18, SENet18, and VGG11.
For each model, we evaluate its three variants: the original model as the baseline, the model accelerated with the LUT-NN method, and the model accelerated with the MADDNESS method.

We will compare LUT-NN models with the original models and MADDNESS models in several aspects, including accuracy, latency, and memory/power consumption.

\subsection{Installation}

LUT-NN has already been installed in the AE server.
Reviewers can log in to the AE server, run the experiments and then review the results.

Besides the AE server, we also list the installation steps below for users that do not have access to the AE server:

\begin{enumerate}
    \item Install \href{https://github.com/lutnn/tvm-dpq}{TVM for LUT-NN} according to the README in the repository.
    \item Install \href{https://github.com/microsoft/onnxruntime/tree/v1.12.1}{ONNX Runtime v1.12.1}  according to the README in the repository.
    \item Install \href{https://github.com/lutnn/blink-mm/tree/main}{LUT-NN} according to the README in the repository.
\end{enumerate}

\subsection{Experiment workflow}
The root README for AE is \url{https://github.com/lutnn/blink-mm/blob/main/blink_mm/ae/readme.md}.

The basic workflow of LUT-NN experiments can be listed below:

\begin{enumerate}
    \item Set up the TVM RPC tracker on the AE server and then set up TVM RPC servers on the Android phones.
    \item Evaluate the latency of models using LUT-NN, TVM, and ONNX Runtime;
    \item Evaluate GOPs (Giga operations) and disk size of LUT-NN models and the original models;
    \item Evaluate the accuracy of LUT-NN models, the MADDNESS models, and the original models;
    \item Evaluate the power and memory of models using LUT-NN and TVM, respectively;
    \item Evaluate the results of ablation studies.
\end{enumerate}

To know the details of the experiment workflow, please refer to the \href{https://github.com/lutnn/blink-mm/tree/main/blink_mm/ae}{AE README} in the \href{https://github.com/lutnn/blink-mm/tree/main}{LUT-NN} repository.

\subsection{Evaluation and expected results}

You will get the exact same GOPs, disk size, and accuracy with the data in table \ref{tab:flops}, table \ref{tab:cnn_accuracy} and table \ref{tab:bert_accuracy}.
Besides, the latency, power, and memory data of the models will be similar to Fig. \ref{fig:layerwise}, table \ref{tab:end_to_end_power}, Fig. \ref{fig:end_to_end_latency}, Fig. \ref{fig:multi_threading}, Fig. \ref{fig:memory}, Fig. \ref{fig:ablation}, Fig. \ref{fig:resnet18_grid_search} and Fig. \ref{fig:bert_num_layers_to_replace}.

\subsection{Experiment customization}

\subsection{Notes}

\subsection{Methodology}

Submission, reviewing and badging methodology:

\begin{itemize}
  \item \url{https://www.acm.org/publications/policies/artifact-review-badging}
  \item \url{http://cTuning.org/ae/submission-20201122.html}
  \item \url{http://cTuning.org/ae/reviewing-20201122.html}
\end{itemize}
